# Supplementary material for: MultLFG: Training-free Multi-LoRA composition using Frequency-domain Guidance
Source: arXiv:2505.20525 source file (2025-05-26)
Supplement: Supplementary file 1 [file X_supple.tex]

\clearpage
\setcounter{page}{1}
\maketitlesupplementary
% \section{Appendix}
%\section{Introduction}

In this supplementary material, we will provide the following details. 
\begin{enumerate}
    \item Training details.
    \item Theoretical and intuitive justification.
    \item Experimental setup.
    \item Image-to-latent scaling.
    
\end{enumerate}

\section{Training details}

We provide the hyperparameters for realistic and anime style in Tab.~\ref{tab:reality_hparams} and Tab.~\ref{tab:anime_hparams}.

\begin{table}[!h]
    \centering
    \caption{Hyperparameters for realistic style}
    \scalebox{1.0}{
    \begin{tabular}{cc}
    \toprule
    Hyperparameter & Values \\
    \midrule
    No. of inference step & 100 \\
    Guidance scale & 7 \\
    Cross-attention scale & 0.8 \\
    Text-to-image diffusion model & Stable Diffusion-v1~\cite{rombach2022high} \\
    Number of DWT components & 4\\
    DWT filter & 'Haar'\\
    \bottomrule
    \end{tabular}}
    \label{tab:reality_hparams}
\end{table}

\begin{table}[!h]
    \centering
    \caption{Hyperparameters for anime style}
    \scalebox{1.0}{
    \begin{tabular}{cc}
    \toprule
    Hyperparameter & Values \\
    \midrule
    No. of inference step & 200 \\
    Guidance scale & 10 \\
    Cross-attention scale & 0.8 \\
    Text-to-image diffusion model & Stable Diffusion-v1~\cite{rombach2022high} \\
    Number of DWT components & 4\\
    DWT filter & 'Haar'\\
    \bottomrule
    \end{tabular}}
    \label{tab:anime_hparams}
\end{table}

\vspace{-0.3cm}
\section{Theoretical and intuitive justification}
\vspace{-0.3cm}

\begin{lemma}[Frequency decomposition reduces interference]
Let \( x \) represent an image composed of multiple concepts \( \{c_i\}_{i=1}^n \). Consider wavelet decomposition of the image into frequency-specific subbands \( b \in \{LL, LH, HL, HH\} \):
$x = \sum_{b \in \{LL,LH,HL,HH\}} x_b.$

Define interference between concepts \( c_i \) and \( c_j \) within a subband \( b \) as:
\[
I_b(c_i, c_j) = \frac{\langle x_b^{c_i}, x_b^{c_j} \rangle}{\|x_b^{c_i}\|_2 \|x_b^{c_j}\|_2}.
\]
Then, interference in the frequency domain is strictly lower than the spatial domain interference:
\[
|I_b(c_i, c_j)| \leq |I_{\text{spatial}}(c_i, c_j)|,
\]
with equality only if \( x_b^{c_i} \) and \( x_b^{c_j} \) perfectly align spatially and frequency-wise.
\end{lemma}

\begin{proof}
Consider the spatial domain representations \( x^{c_i} \) and \( x^{c_j} \) for two distinct concepts \( c_i \) and \( c_j \). By the Cauchy–Schwarz inequality:
\[
|\langle x^{c_i}, x^{c_j} \rangle| \leq \|x^{c_i}\|_2 \|x^{c_j}\|_2.
\]
Equality holds only when \( x^{c_i} \) and \( x^{c_j} \) are linearly dependent. After wavelet decomposition, the spatial domain vectors are partitioned into frequency-specific vectors \( x_b^{c_i} \) and \( x_b^{c_j} \). Thus:
\[
|\langle x_b^{c_i}, x_b^{c_j} \rangle| \leq \|x_b^{c_i}\|_2 \|x_b^{c_j}\|_2.
\]
Because wavelet decomposition distributes the original spatial features into separate subbands, reducing direct spatial overlap, it follows that:
\[
|I_b(c_i, c_j)| = \frac{|\langle x_b^{c_i}, x_b^{c_j} \rangle|}{\|x_b^{c_i}\|_2 \|x_b^{c_j}\|_2} \leq \frac{|\langle x^{c_i}, x^{c_j} \rangle|}{\|x^{c_i}\|_2 \|x^{c_j}\|_2} = |I_{\text{spatial}}(c_i, c_j)|.
\]
Equality is only achieved when \( x_b^{c_i} \) and \( x_b^{c_j} \) precisely align in both frequency and spatial domains, which is highly unlikely in practice due to the nature of wavelet decomposition.
\end{proof}

\section{Experimental setup.}

We conduct our experiments using the ComposeLoRA testbed~\cite{zhong2024multi}, which includes two subsets of LoRAs representing realistic and anime styles. Each subset consists of 22 LoRAs spanning 3 characters, 2 clothing types, 2 styles, 2 backgrounds, and 2 objects. The evaluation involves 480 unique composition sets, categorized as 48 sets with 2 LoRAs, 144 sets with 3 LoRAs, 192 sets with 4 LoRAs, and 96 sets with 5 LoRAs. To maintain compositional consistency, each set includes one character LoRA, ensuring no category overlaps. 
Following ComposeLoRA~\cite{zhong2024multi}, we use the composeLoRA testbed for our experiments. It consists of two unique subsets of LoRAs representing realistic and anime styles. Each subset comprises a variety of elements: 3 characters, 2 types of clothing, 2 styles, 2 backgrounds, and 2 objects, culminating in a total of 22 LoRAs in ComposLoRA. Thus, the ComposLoRA evaluation incorporates a total of 480 distinct composition sets. This includes 48 sets comprising 2 LoRAs, 144 sets with 3 LoRAs, 192 sets featuring 4 LoRAs, and 96 sets containing 5 LoRAs. It was make sure that each set include one character LoRA and avoid duplication of element categories to prevent conflicts.

To evaluate the composition of concepts, we use CLIP-score~\cite{zou2025cached} as an evaluation metric, which measure the alignment between text and images. Although existing metrics can measure the alignment between text and images, they often lack the nuance needed to assess the finer details of specific elements within an image and the overall quality of their composition. Recently, multimodal large language models like GPT-4V have demonstrated strong performance across a range of multimodal tasks, highlighting their potential for evaluating image generation. In this work, we harness GPT-4V’s capabilities to serve as an evaluator for composable image generation. We adopt a comparative evaluation strategy in which GPT-4V rates generated images along two dimensions: composition quality and image quality. Each image is scored on a scale from 0 to 10, with higher scores reflecting better quality. To guide the evaluation, GPT-4V is provided with a prompt containing the key attributes of the target composition, clear scoring criteria for both dimensions, and an expected response format. Full details of the evaluation prompts and results can be found in the Appendix. This setup enables a systematic comparison of our proposed methods against the LoRA Merge, LoRA-switch, and LoRA-composite baselines.

\textbf{User study.} Since perceptual metrics are not always reliable, we also conducted a human preference study using Amazon Mechanical Turk (AMT) for assesing the compositionality and quality. We asked 50 unbiased users rank our method against
baselines, totaling 1000 questionnaires. The aggregate responses showed that MultLFG generated images significantly outperformed baselines.

\section{Image-to-latent scaling}
The detailed algorithm for image-to-latent scaling is provided in Alg.~\ref{alg:img2latent}.

\begin{algorithm}[!t]
\caption{Img2Latent : Image Delta to Latent Delta Transform}\label{alg:img2latent}
\begin{algorithmic}

\State \textbf{Input:} Image $x\in\mathbb{R}^{H\times W\times C}$, Wavelet-domain perturbation $\Delta \hat{x} = \left( \Delta x_{LL}, \Delta x_{HL}, \Delta x_{LH}, \Delta x_{HH} \right)$, Encoder $E(\cdot)$ (e.g., VAE encoder), Inverse wavelet transform $\text{IDWT}$, Perturbation magnitude $\epsilon > 0$

\State \textbf{Output:} Latent-space delta $\Delta z$ and, optionally, its decomposition $\left( \Delta z_{LL}, \Delta z_{HL}, \Delta z_{LH}, \Delta z_{HH} \right)$
\medskip

\State \textbf{1. Reconstruct the Image-Space Perturbation:}
\State Compute $\Delta x \gets \text{IDWT}(\Delta \hat{x})$, where
\[
\Delta \hat{x} = (\Delta x_{LL}, \Delta x_{HL}, \Delta x_{LH}, \Delta x_{HH})
\]
\medskip
\State \textbf{2. Compute the Baseline and Perturbed Latent Codes:}
\State Compute baseline latent code: $z \gets E(x)$.
\State Compute perturbed latent code: $z' \gets E(x + \Delta x_{\mathcal{F}})$.

\medskip
\State \textbf{3. Compute the Latent Delta via Finite Difference:}
\State Compute the latent difference:
\[
\Delta z \gets \frac{z' - z}{\epsilon}
\]
\medskip
\State \textbf{4. Decompose $\Delta z$ into Latent Subbands:}

\hspace{0.4cm} \For{latent subbands $i\in\{\text{LL}, \text{HL}, \text{LH}, \text{HH}\}$}{
    \State Apply projection: $\Delta z_i \gets P_i(\Delta z)$.}
\EndFor
\medskip
\State \textbf{5. Importance of Concepts in Latent space:} \[\bar{w}_{\mathcal{F}} = \sum_{\mathcal{F'} \in \{\mathrm{LL}, \mathrm{HL}, \mathrm{LH}, \mathrm{HH}\}} w_{\mathcal{F'}} * \Delta z_\mathcal{F} \]

\State \Return $\bar{w}$ 
\end{algorithmic}
\end{algorithm}
